# Supplementary material for: Multi-set variational quantum dynamics algorithm for simulating nonadiabatic dynamics on quantum computers
Source: arXiv:2503.07388 source file (2025-03-10)
Supplement: Supplementary file 1 [file si.pdf]

# Supporting Information: Multi-set variational quantum dynamics algorithm for simulating nonadiabatic dynamics on quantum computers

Jingjing Li,[†] Weitang Li,[‡] Xiaoxiao Xiao,[†] Limin Liu,[†] Zhendong Li,[†] Jiajun Ren,[*,†] and Weihai Fang[†]

†*Key Laboratory of Theoretical and Computational Photochemistry, Ministry of Education, College of Chemistry, Beijing Normal University, Beijing 100875, People's Republic of China*

‡*School of Science and Engineering, The Chinese University of Hong Kong, Shenzhen, 518172, P. R. China.*

E-mail: jjren@bnu.edu.cn

## 1. Measurements of $\mathbf{A}, \mathbf{B}, \mathbf{D}, \mathbf{H}$ in MS-VQD

The expression for one parameterized quantum circuit (PQC) is

$$\chi_p = U(\vec{\theta}^p)|\mathbf{0}\rangle = U_n U_{n-1} \cdots U_1 |\mathbf{0}\rangle, \tag{1}$$

where the label $p$ in $U_k$ is omitted for clarity. If $U_k$ contains parameter $\theta_k$,

$$\frac{\partial \chi_p}{\partial \theta_k} = U_n \cdots U_{k+1}(\sum_j \alpha_j O_j)U_{k-1} \cdots U_1|\mathbf{0}\rangle, \tag{2}$$

where $\alpha_j$ is a complex number, $O_j$ is an unitary operation. For $U_k = e^{i\theta_k \sigma_k}$, where $\sigma_k$ is a pauli string, $\frac{\partial U_k}{\partial \theta_k} = i\sigma_k U_k = iU_k\sigma_k$. Thus, only one term exists $\alpha = i$, $O = \sigma_k U_k$. We only consider this simple case below, the generalization to multiple terms is straightforward. After the decomposition in eq (2), the measurement of $D_k^{pp}$ is

$$D_k^{pp} = \langle \frac{\partial \chi_p}{\partial \theta_k}|\chi_p\rangle = -i\langle 0|U_1^\dagger \cdots U_{k-1}^\dagger \sigma_k^\dagger U_{k-1} \cdots U_1|0\rangle \tag{3}$$

Because the bra and ket are the same, which is $U_{k-1} \cdots U_1|0\rangle$, this expression can be measured with the circuit shown in Figure S1(a). Similarly,

$$A_{lk}^{pp} = \langle \frac{\partial \chi_p}{\partial \theta_l^p}|\frac{\partial \chi_p}{\partial \theta_k^p}\rangle = \langle 0|U_1^\dagger \cdots U_{l-1}^\dagger \sigma_l^\dagger U_l^\dagger \cdots U_{k-1}^\dagger \sigma_k U_{k-1} \cdots U_1|0\rangle, \quad l < k \tag{4}$$

To measure $A_{lk}^{pp}$, only $\sigma_l$ and $\sigma_k$ has to be controlled by the ancilla qubit in Hadamard test as VQD.[?] The circuit is shown in Figure S1(b).

$$H_{pq} = \langle \chi_p|\hat{T} + \hat{V}_{pq}|\chi_q\rangle = \langle 0|U_1^\dagger \cdots U_n^\dagger(\hat{T} + \hat{V}_{pq})V_n \cdots V_1|0\rangle \tag{5}$$

$$B_l^{pq} = \langle \frac{\partial \chi_p}{\partial \theta_l^p}|\hat{T} + \hat{V}_{pq}|\chi_q\rangle = -i\langle 0|U_1^\dagger \cdots U_{l-1}^\dagger \sigma_l^\dagger U_l^\dagger \cdots U_n^\dagger(\hat{T} + \hat{V}_{pq})V_n \cdots V_1|0\rangle \tag{6}$$

The operator $(\hat{T} + \hat{V}_{pq})$ can be further decomposed into a sum of pauli strings. To measure $H_{pq}$ and $B_l^{pq}$, all gates where $U_k$ and $V_k$ are not equal should be controlled by the ancilla qubit in Hadamard test, which is more complicated than traditional VQD. The circuits are shown in Figure S1(c) and (d).

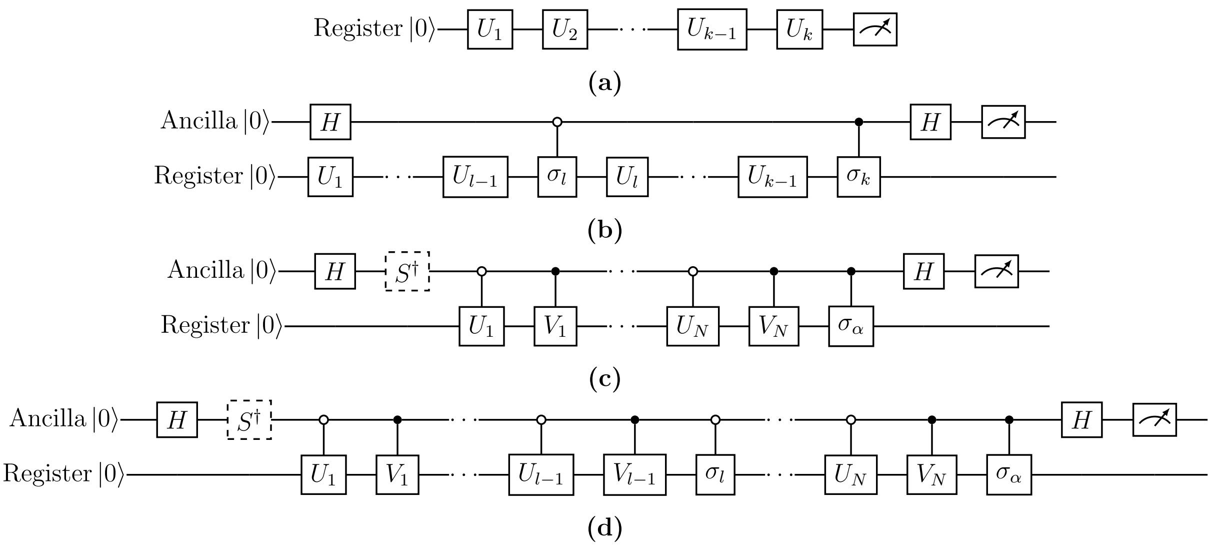


Figure S1: The circuits for measurement. (a) $D_k^{pp}$ (b) Re$A_{lk}^{pp}$ (c) $H_{pq}$ (d) $B_l^{pq}$ .

# 2. The number of Hamiltonian terms after mapping to qubit operators

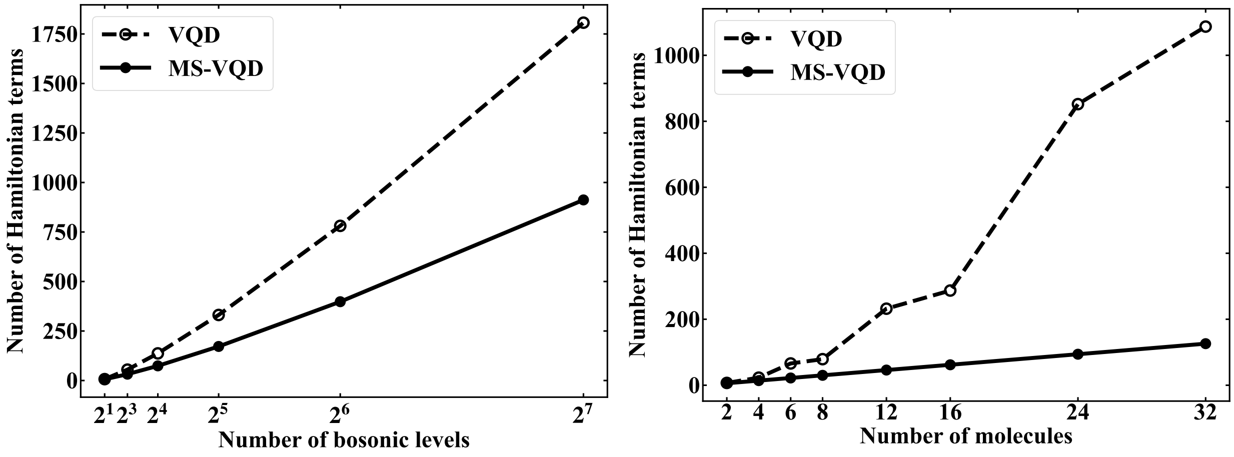


(a) (b)

Figure S2: The number of Hamiltonian terms with (a) the number of local bosonic levels $d$ (dimer $N = 2$) and with (b) the number of molecules $N$ (bosonic levels $d = 2$) after mapping to qubits.

The number of Hamiltonian terms in VQD is much larger than that of MS-VQD, because the mapping of electronic operators into qubits in VQD using binary/gray code leads to a overhead prefactor, which is approximately linear with the number electronic states. In this regard, using unary code to encode electronic state in VQD is better to save the number of measurements.

## 3. The population dynamics with RyRz-full-Rzz ansatz and XYZ2F ansatz

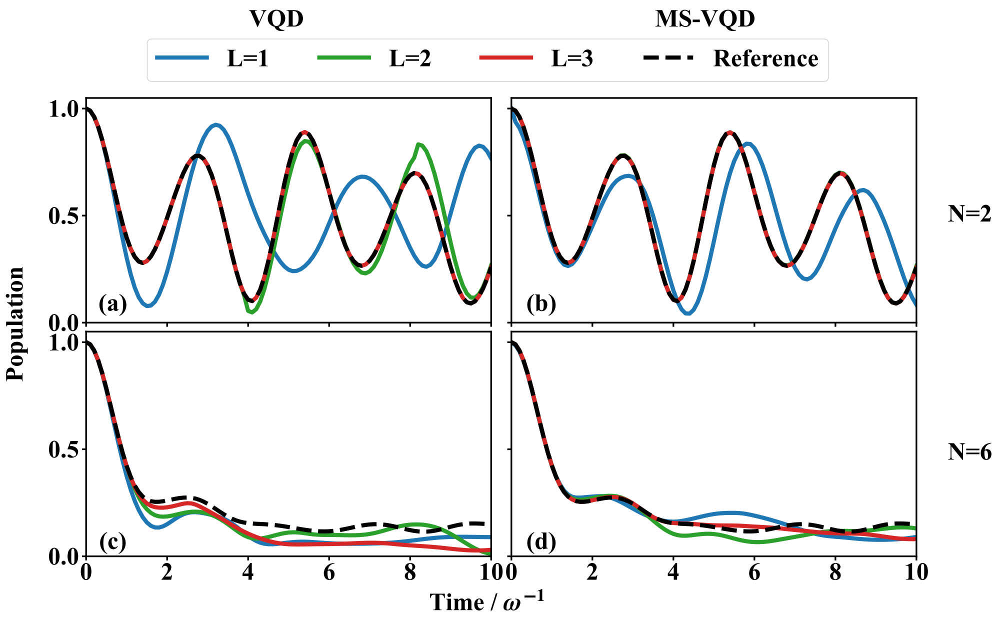


Figure S3: The exciton population on the first molecule with time $|\langle\phi_1|\Psi(t)\rangle|^2$. (a)(b) The result of VQD (a) and MS-VQD (b) for dimer model. Different colors represent different layers of ansatz $L = 1, 2, 3$. The dashed black curve is the reference results calculated by the time-dependent density matrix renormalization group algorithm. (c)(d) Same as (a)(b) but for hexamer. The RyRz-full-Rzz ansatz is used.

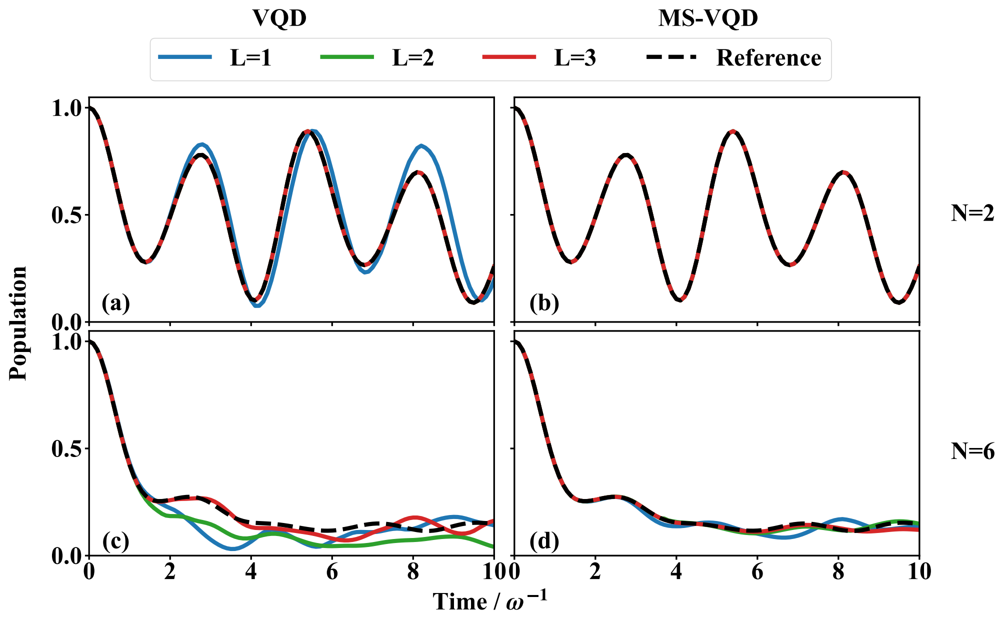


Figure S4: Same as Figure S3 but with XYZ2F ansatz.

# 4. Infidelity as a function of the number of ansatz layers

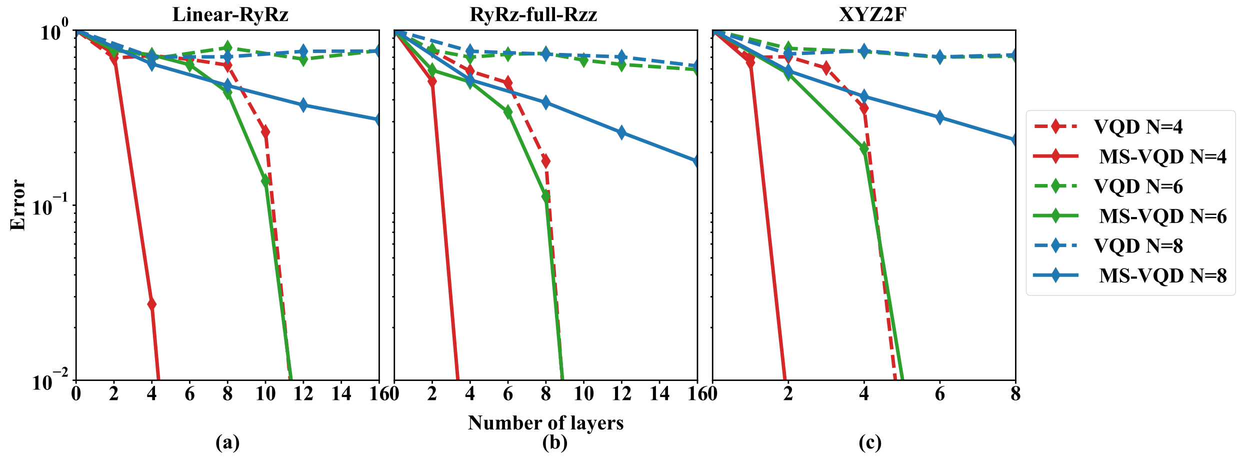


Figure S5: The infidelity $1 - \mathrm{Re}\langle\Psi^{\mathrm{ref}}(t)|\Psi(t)\rangle$ with different layers of ansatz by VQD and MS-VQD. (a) linear-RyRz ansatz (b) RyRz-full-Rzz ansatz (c) XYZ2F ansatz. Different colors indicate different system sizes.

# 5. The number of parameters in VQD and MS-VQD

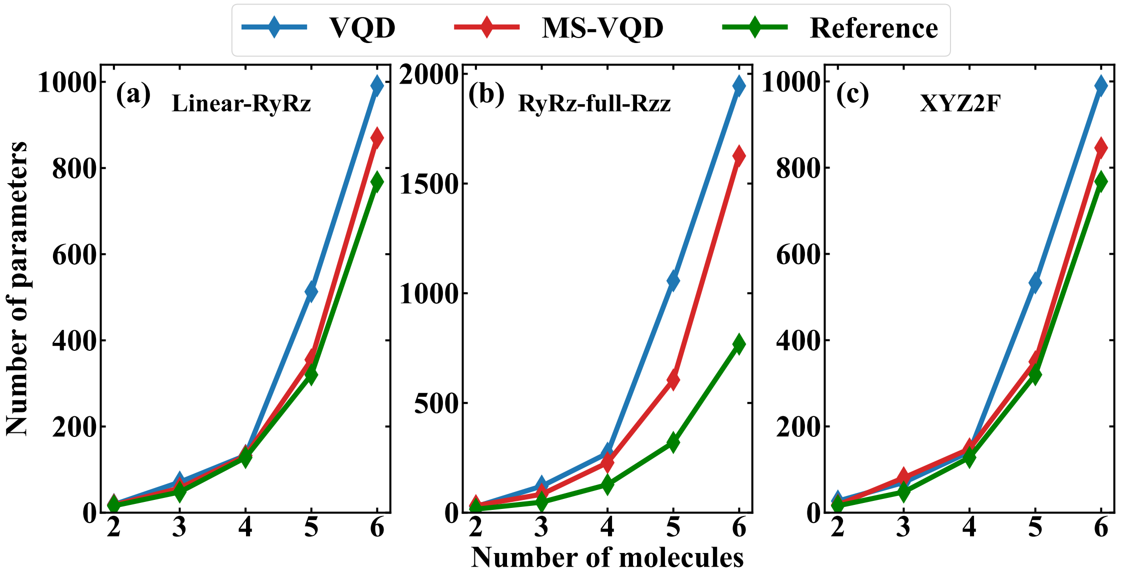


Figure S6: The total number of parameters in VQD and MS-VQD to achieve error less than $10^{-3}$ for different number of molecules from 2 to 6. (a) linear-RyRz ansatz (b) RyRz-full-Rzz ansatz (c) XYZ2F ansatz. The size of full Hilbert space is also plotted as reference.

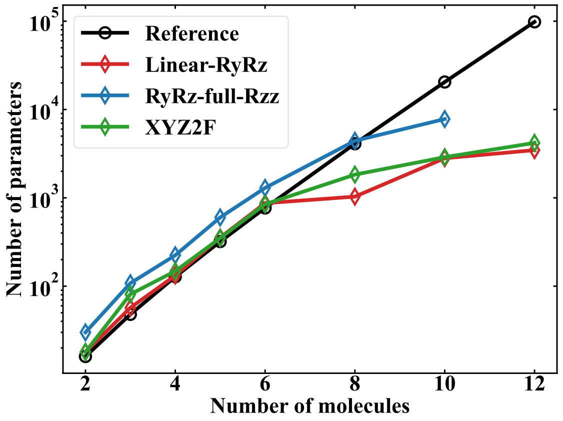


Figure S7: The total number of parameters in MS-VQD to achieve error less than $10^{-3}$ for different system sizes. The size of full Hilbert space is also plotted as reference.

# 6. The performance of MS-VQD and VQD with different coupling strength and number of modes

We evaluated the performance of MS-VQD for different values of the electronic coupling constant $J$, electron-vibration coupling constant $g$, and different number of modes in a dimer. Figure S8 shows that the accuracy of MS-VQD remains similar across different parameter regimes when the number of layers is fixed, demonstrating that the advantage of MS-VQD over VQD holds in wide coupling regimes. For systems with varying numbers of vibrational modes, the vibrational frequency and electron-vibration coupling are $\omega \in [1/N, 2/N, \cdots, 1]$, $g = \sqrt{1/\sum_i \omega_i^2}$ (the total reorganization energy is fixed to be 1). Figure S9 illustrates that as the number of vibrational modes increases, the required number of ansatz layers must also increase to maintain accuracy. Notably, the advantage of MS-VQD over VQD remains robust with different number of vibrational modes.

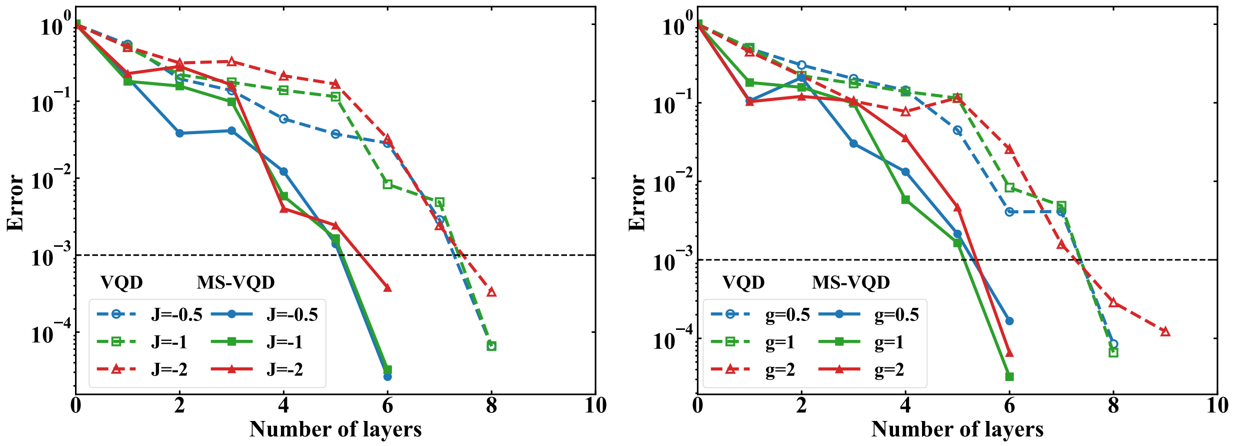


(a) (b)

Figure S8: The error with different number of ansatz layers by VQD and MS-VQD under (a) different excitonic coupling $J$ and (b) electron-vibration coupling $g$. Linear-RyRz ansatz is used.

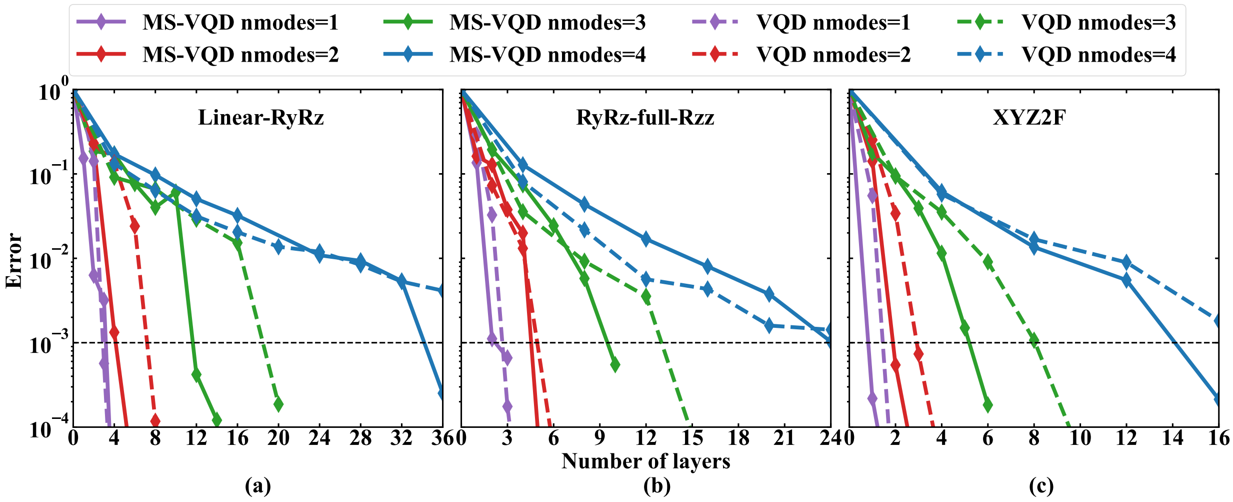


Figure S9: The error of population with different layers of ansatz by VQD and MS-VQD. (a) linear-RyRz ansatz (b) RyRz-full-Rzz ansatz (c) XYZ2F ansatz. Different colors indicate different number of modes.

# References


(S) Yuan, X.; Endo, S.; Zhao, Q.; Li, Y.; Benjamin, S. C. Theory of variational quantum simulation. *Quantum* **2019**, *3*, 191.
